# Supplementary material for: Zeroth order regular approximation approach to electric dipole moment interactions of the electron
Source: arXiv:1703.06838 ancillary file (2017-03-09)
Supplement: Supplementary file 1 [file suppl.pdf]

# Supplemental Material for "Zeroth order regular approximation approach to electric dipole moment interactions of the electron"

Konstantin Gaul and Robert Berger

*Fachbereich Chemie, Philipps-Universität Marburg, Hans-Meerwein-Straße 4, 35032 Marburg, Germany*

(Dated: March 9, 2017)

## I. BASIS SETS

Table I. Basis set parameters for GHF/GKS-ZORA calculations. Even-tempered basis sets of uncontracted Gaussians are given in the form $N_{\text{bas}}\ell$: ($\alpha_{\text{max}}$; $\alpha_{\text{min}}$), where $N_{\text{bas}}$ is the number of Gaussians, $\ell$ is the symbol for the angular momentum quantum numbers and $\alpha_{\text{max}}$ and $\alpha_{\text{min}}$ are the largest and smallest exponent coefficients, respectively, given in units of $a_0^{-2}$ with $a_0$ being the Bohr radius.

| Basis for all 'heavy' centers | F ANO basis | | |
|---|---|---|---|
| | s | p | d |
| 37s: (2000000000; 0.0291) | 103109.46 | 245.33029 | 5.000000 |
| 34p: (500000000; 0.0582) | 15281.007 | 56.919005 | 1.750000 |
| 14d: (13300.758; 0.0521) | 3441.5392 | 17.604568 | 0.612500 |
| 9f: (751.8368350; 0.3546) | 967.09483 | 6.2749950 | 0.214375 |
| | 314.03534 | 2.4470300 | |
| | 113.44230 | 0.9950600 | |
| | 44.644727 | 0.4039730 | |
| | 18.942874 | 0.1548100 | |
| | 8.5327430 | 0.0541840 | |
| | 3.9194010 | | |
| | 1.5681570 | | |
| | 0.6232900 | | |
| | 0.2408610 | | |
| | 0.0843010 | | |
